# Supplementary material for: Optimization of a solid-state electron spin qubit using Gate Set Tomography
Source: arXiv:1606.02856 ancillary file (2016-06-16)
Supplement: Supplementary file 2 [file GSTreport_fig2cd.pdf]

# GST report for data\_fig2c-d

March 29, 2016

## 1 Overview

This report presents a gate-set tomography (GST) analysis of a dataset called “data\_fig2c-d”.

GST characterizes logic operations on a quantum device (e.g., a qubit), by treating it as a black box. This black box is equipped with a small set of “buttons” that apply quantum *gates* to the quantum system inside. One button initializes it, a second button triggers a 2-outcome measurement, and the remaining buttons perform transformations. We avoid assumptions about the device’s operation whenever possible. Currently, we assume that:

- the quantum device is a qubit (has a Hilbert space of dimension 2),
- each *gate*, or logic operation, can be represented by a stationary Markov process (a.k.a. “quantum channel”).

The core of GST is an algorithm that takes certain inputs, and produces certain outputs. The *input* to GST comprises (1) a list of data, and (2) “target” gateset describing the *ideal* behavior of the device. GST data comprises a list of experiments – each described by the sequence of gates that was applied – and, for each experiment, two integer *counts* stating how often the “plus” and “minus” results were observed. The target gates are used *only* to (a) report how consistent the estimates are with the target, and (b) choose the best *gauge* in which to report the results. GST does not take them into account in its core analysis, and there is no possibility of circularity or other “cheating”.

GST’s primary output is an estimated *gateset* that models or fits the device’s observed behavior. Gatesets are of the form  $\{\rho_0, E_0, \{G_k\}\}$ , where

- $\rho_0$  is an estimate of the density matrix in which the device gets initialized,
- $\{E_0, \mathbb{1} - E_0\}$  is an estimate of the POVM describing how it gets measured,
- and each of the  $G_k$  is an estimate of the superoperator (quantum process) describing the corresponding gate.

Unless something went wrong (usually it doesn’t), the output of GST is the best possible fit to the data. This should also mean that they are a very accurate description of what happens when you trigger a gate on your device. However, this happy conclusion relies on two assumptions:

1. The experiments were chosen wisely, so that the only gate sets consistent with their results are very close to the true behavior. This is usually true. The main failure mode occurs when you were not able to perform *long* sequences (e.g., because your decoherence rate is very high), in which case accuracy may be limited.
2. The operations you are performing really are stationary (time-independent), Markovian, and acting on a quantum system with the correct Hilbert space dimension. These assumptions define the *model* that GST fits to the data. **They are usually not true!** Quantum operations are usually at least a little bit non-Markovian. In this report (Section 4) we provide extensive self-checks to identify and diagnose violations of the model. If your system *is* visibly non-Markovian, then (a) these checks will probably warn you of it, and (b) the other quantities reported here should be treated with caution – using GST on non-Markovian gates violates the warranty!

This document is organized into three main sections, which address three broad questions.

- Section 2: What inputs did you give GST?
- Section 3: What estimate did GST output, and what does it mean?
- Section 4: How reliable are the results? (How badly was the model violated?)

Section 2 is primarily useful to verify that the inputs were correct. Section 3 is the most important: it presents the raw estimates derived by the GST algorithm, and also provides a variety of derived quantities that may be useful in interpreting what this estimate means.

Section 4) is dedicated to summarizing how well the model imposed by GST was able to fit the data, relative to what is expected of a “good” model. This is *not* related to “How close is the GST estimate to the target gates?”, which is addressed in Section 3. It is also not the same as “How large are the error bars on the GST estimate?”, which is a good question that we do not directly address at this time. Instead, Section 4 is intended to tell you whether (a) you should take the GST estimate at face value, or (b) it should be treated skeptically because *no* gate set was capable of fitting the data.

Finally, appendices may be present (depending on which options were chosen when this report was generated). Appendices present more detailed debugging information, elaborating on the goodness-of-fit metrics presented in Section 4.

## 2 Input Summary

The input for this GST analysis comprised: (1) a target gateset (see Tables 1-2); and (2) a dataset called “data\_fig2c-d”.

### 2.1 Target Gateset

The target gateset describes the ideal initial state (density matrix), measurement (POVM effect), and gate operations (superoperators). Typically, density matrices and POVM effects are represented as square  $d \times d$  matrices on a Hilbert space  $\mathcal{H}$ . In GST, it is often more convenient to represent them as  $d^2$ -element vectors in the Hilbert-Schmidt space  $\mathcal{B}(\mathcal{H})$  of linear operators on  $\mathcal{H}$ . Both representations are shown in Table 2. Superoperators are sometimes represented in Choi or Kraus form, but for GST it is more convenient to represent them as square  $d^2 \times d^2$  matrices that multiply associatively and act on  $\mathcal{B}(\mathcal{H})$ . These are shown in Table 2.

These Hilbert-Schmidt space representations require choosing a basis  $\{M_i\}$  for  $\mathcal{B}(\mathcal{H})$ . We use the *Pauli basis*, comprising the four  $2 \times 2$  Pauli matrices (including the identity  $\mathbb{1}$ ) for  $d = 2$ . In  $d > 2$ , we use the analogous Gell-Mann matrices as a basis. The choice of this basis is what is meant when state preparations and measurements are written as vectors and gate operations are written as matrices in the “Pauli basis”. Keep in mind that we want to use an orthonormal basis, so the basis matrices are normalized so that  $\langle\langle M_i | M_j \rangle\rangle = \text{Tr} M_i^\dagger M_j = \delta_{ij}$ . In  $d = 2$ , this means that the basis matrices are  $M_i = \frac{1}{\sqrt{2}} \sigma_i$ .

The ideal SPAM operations for your particular case are given in Table 1. The ideal *logic gate* operations are given, as superoperators written in the Pauli basis, in Table 2.

In most cases, the ideal/target logic gates are reversible unitary rotations. The corresponding superoperators are orthogonal rotations on  $\mathcal{B}(\mathcal{H})$ . For your convenience, Table 2 also lists (for each logic gate) an axis of rotation [as a vector in  $\mathcal{B}(\mathcal{H})$ ] and an angle of rotation.

### 2.2 GST Input Data

The most important input to GST is a *dataset* – a list of experimental counts or frequencies, each associated with a *gate sequences*. Gate sequences are also referred to as “gate strings”. Each gate sequence defines an experiment, in which you (1) initialize the device, (2) apply the operations specified by the gate sequence, and (3) measure and record the result (“plus” or “minus”).

Typically, the gate sequences that appear in the dataset are generated by the following process:

1. A small set of short gate sequences called *germs* are chosen,

| Operator | Hilbert-Schmidt vector (Pauli basis) | Matrix                                         |
|----------|--------------------------------------|------------------------------------------------|
| $\rho$   | 0.7071                               | $\begin{pmatrix} 1 & 0 \\ 0 & 0 \end{pmatrix}$ |
|          | 0                                    |                                                |
|          | 0                                    |                                                |
|          | 0.7071                               |                                                |
| $E$      | 0.7071                               | $\begin{pmatrix} 0 & 0 \\ 0 & 1 \end{pmatrix}$ |
|          | 0                                    |                                                |
|          | 0                                    |                                                |
|          | -0.7071                              |                                                |

Table 1: **Target gateset: SPAM (state preparation and measurement) gates.** These are the *ideal* input state ( $\rho_0$ ) and ‘plus’ POVM effect  $E_0$  for the device on which we report. SPAM gates are given here both as  $d \times d$  matrices, and in “vectorized” form as  $d^2$ -dimensional vectors in  $\mathcal{B}(\mathcal{H})$ . See Table 5 for GST estimates of the actual  $\rho_0$  and  $E_0$  implemented in this experiment.

| Gate | Superoperator (Pauli basis)                                                                       | Rotation axis | Angle    |
|------|---------------------------------------------------------------------------------------------------|---------------|----------|
| Gi   | $\begin{pmatrix} 1 & 0 & 0 & 0 \\ 0 & 1 & 0 & 0 \\ 0 & 0 & 1 & 0 \\ 0 & 0 & 0 & 1 \end{pmatrix}$  | 0             | $0\pi$   |
|      |                                                                                                   | 1             |          |
|      |                                                                                                   | 0             |          |
|      |                                                                                                   | 0             |          |
| Gx   | $\begin{pmatrix} 1 & 0 & 0 & 0 \\ 0 & 1 & 0 & 0 \\ 0 & 0 & 0 & -1 \\ 0 & 0 & 1 & 0 \end{pmatrix}$ | 0             | $0.5\pi$ |
|      |                                                                                                   | 1             |          |
|      |                                                                                                   | 0             |          |
|      |                                                                                                   | 0             |          |
| Gy   | $\begin{pmatrix} 1 & 0 & 0 & 0 \\ 0 & 0 & 0 & 1 \\ 0 & 0 & 1 & 0 \\ 0 & -1 & 0 & 0 \end{pmatrix}$ | 0             | $0.5\pi$ |
|      |                                                                                                   | 0             |          |
|      |                                                                                                   | 1             |          |
|      |                                                                                                   | 0             |          |

Table 2: **Target gateset: logic gates.** These are the *ideal* (generally unitary) logic gates. Each has a name starting with “G”, and is represented as a  $d^2 \times d^2$  *superoperator* that acts by matrix multiplication on vectors in  $\mathcal{B}(\mathcal{H})$ . For each gate, its axis of rotation (in  $\mathcal{B}(\mathcal{H})$ ) and angle of rotation are also given. See Table 7 for GST estimates of the actual logic gates implemented in this experiment.

2. A small set of short *fiducial sequences* are chosen so that, when applied to  $\rho_0$  or  $E_0$ , they generate an informationally complete set of states or effects.
3. Each germ is concatenated with itself to form *base sequences* of length approximately  $1, 2, 4, 8, \dots L_{max}$ .
4. Each base sequence is sandwiched between every possible pair of fiducial sequences.

The dataset comprises all sandwiched base sequences. A few other short sequences (e.g., those corresponding to the empty base sequence) may also appear.

The fiducial sequences and germs for *this* dataset are given in Table 3. An overview of the information contained in the file you provided for dataset “data\_fig2c-d” is given in Table 4.

This table also contains one derived quantity, the spectrum of the largest *Gram matrix* that GST could extract from the data. This is included here rather than in the analysis because it is not useful for predictive purposes, and therefore is not part of the estimate. It serves, instead, to tell you something about the quality of the data. More precisely, it tells you about the dimension of the state space that is explored by the fiducial sequences. This should be  $d^2$ -dimensional [because the fiducials are intended to explore all of  $\mathcal{B}(\mathcal{H})$ ], and therefore the spectrum listed in Table 4 should (ideally) have exactly  $d^2$  elements that are large and nonzero. In practice, you should see  $d^2$  large elements, and a rapid drop in magnitude thereafter. If fewer than  $d^2$  elements are large, then the fiducials were poorly chosen and are not exploring the state space effectively. If

more than  $d^2$  are large, then the system is experiencing strong non-Markovian effects (e.g., strong coupling to environmental degrees of freedom) or it has a larger Hilbert space dimension than expected.

| Fiducials |              |              | #  | Germ                        |
|-----------|--------------|--------------|----|-----------------------------|
| #         | Prep.        | Measure      |    |                             |
| 1         |              |              | 1  | Gx                          |
| 2         | Gx           | Gx           | 2  | Gy                          |
| 3         | Gy           | Gy           | 3  | Gi                          |
| 4         | Gx · Gx      | Gx · Gx      | 4  | Gx · Gy                     |
| 5         | Gx · Gx · Gx | Gx · Gx · Gx | 5  | Gx · Gy · Gi                |
| 6         | Gy · Gy · Gy | Gy · Gy · Gy | 6  | Gx · Gi · Gy                |
|           |              |              | 7  | Gx · Gi · Gi                |
|           |              |              | 8  | Gy · Gi · Gi                |
|           |              |              | 9  | Gx · Gx · Gi · Gy           |
|           |              |              | 10 | Gx · Gy · Gy · Gi           |
|           |              |              | 11 | Gx · Gx · Gy · Gx · Gy · Gy |

Table 3: **Fiducial sequences and germs.** See discussion in text.

| Quantity           | Value       |
|--------------------|-------------|
| Number of strings  | 2737        |
| Gate labels        | Gx, Gy, Gi  |
| SPAM labels        | plus, minus |
| Gram singular vals | 0.0117      |
|                    | 0.1062      |
|                    | 0.7481      |
|                    | 0.8251      |
|                    | 0.8538      |
|                    | 3.0376      |

Table 4: **General dataset properties.** See discussion in text.

### 3 Output from GST

The primary output of GST is an estimated gateset. This section presents the raw estimate, and then some useful derived quantities of the estimated gates, including comparisons to the target gates.

#### 3.1 Raw GST estimates

Table 5 reports the estimated SPAM operations, and Table 7 reports the logic gate operations. The estimated SPAM gates ( $\rho_0$  and  $E_0$ ) are vectors in  $\mathcal{B}(\mathcal{H})$ , and the estimated logic gates are superoperators represented as matrices acting on  $\mathcal{B}(\mathcal{H})$ , all in the Pauli basis. By taking the dot product of state preparation and measurement vectors estimated SPAM probabilities are computed in Table 6.

The estimated gates can be compared directly to the target gateset given in Section 2. Ideally, they would match. In practice, of course, they won't. One of the best ways we have found to evaluate the significance of discrepancies is to compare *derived* quantities – i.e., certain properties calculated from the gate matrices and SPAM vectors. Deriving quantities from these raw outputs occupies the remainder of this section.

#### 3.2 Derived quantities

Generally, the first thing that you want to know is “How far from ideal are the gates?” To answer this, this report tabulates several well-known metrics of distance. Table 8 lists the discrepancy from each estimated

| Operator | Hilbert-Schmidt vector (Pauli basis)    | Matrix                                                                              |
|----------|-----------------------------------------|-------------------------------------------------------------------------------------|
| $\rho$   | 0.7071<br>0.0191<br>0.0235<br>0.6529    | $\begin{pmatrix} 0.9616 & 0.0214e^{-i0.9} \\ 0.0214e^{i0.9} & 0.0384 \end{pmatrix}$ |
| $E$      | 0.7275<br>-0.0053<br>-0.0032<br>-0.6546 | $\begin{pmatrix} 0.0515 & 0.0043e^{i2.6} \\ 0.0043e^{-i2.6} & 0.9773 \end{pmatrix}$ |

Table 5: **The GST estimate of the SPAM operations.** Compare to Table 1.

|        | $E$     | $E_C$   |
|--------|---------|---------|
| $\rho$ | 0.08686 | 0.91314 |

Table 6: **GST estimate of SPAM probabilities.** Computed by taking the dot products of vectors in Table 5.

| Gate | Superoperator (Pauli basis)                                                                                                                                                |
|------|----------------------------------------------------------------------------------------------------------------------------------------------------------------------------|
| Gi   | $\begin{pmatrix} 1 & 0 & 0 & 0 \\ 0.0001 & 0.9788 & -0.0135 & 0.0021 \\ -0.0002 & 0.0253 & 0.9855 & -0.0016 \\ 0.0002 & 0.0036 & -0.0009 & 0.9992 \end{pmatrix}$           |
| Gx   | $\begin{pmatrix} 1 & 0 & 0 & 0 \\ 5 \times 10^{-6} & 1 & 0.0021 & -0.0005 \\ -0.0002 & 0.0034 & 0.0025 & -0.9972 \\ -0.0002 & -0.0008 & 0.9977 & -0.0019 \end{pmatrix}$    |
| Gy   | $\begin{pmatrix} 1 & 0 & 0 & 0 \\ -0.0002 & -0.0023 & 0.0032 & 0.996 \\ -2 \times 10^{-5} & 0.0042 & 1.0002 & 0.0003 \\ 0.0002 & -0.9955 & -0.0013 & -0.005 \end{pmatrix}$ |

Table 7: **The GST estimate of the logic gate operations.** Compare to Table 2.

gate to its corresponding target, as measured by:

- Process infidelity.** Infidelity is simply  $1 - F$ , where  $F$  is a *fidelity*. The process fidelity between quantum processes  $G_a$  and  $G_b$  is given by  $F = \text{Tr} \left( \sqrt{\sqrt{\chi_a} \chi_b \sqrt{\chi_a}} \right)^2$ , where  $\chi_a$  and  $\chi_b$  are the Jamiolkowski states (normalized Choi process matrices) corresponding to gate matrices  $G_a$  and  $G_b$  respectively. If the target is unitary (as is often the case),  $F = \text{Tr}(\chi_a \chi_b)$ . Process infidelity is roughly what is measured in randomized benchmarking protocols; it quantifies the *incoherent* error rate if coherent errors (e.g. over rotations) are not allowed to accumulate.
- Trace distance.** This is the *Jamiolkowski trace distance* between the Jamiolkowski states corresponding to the two processes:  $d_{tr} = |\chi_a - \chi_b|_1 = \text{Tr} \left( \sqrt{(\chi_a - \chi_b)^2} \right)$ . This distance is useful primarily as a proxy for the *diamond norm distance*, because  $d_{tr} \leq d_\diamond \leq \dim(\mathcal{H}) d_{tr}$ . The diamond norm distance is an upper bound on the rate of error under any possible circumstance (including coherent accumulation of errors) and is often used in proofs of fault tolerance. For gates dominated by coherent/unitary error, it is common to see  $d_\diamond \approx \sqrt{1 - F}$ . For gates dominated by incoherent error,  $d_\diamond \approx 1 - F$ .
- Diamond Norm.** The diamond norm between two quantum processes  $G_a$  and  $G_b$  is given by  $\|G_a - G_b\|_\diamond = \sup_\rho \|(G_a \otimes I_k)(\rho) - (G_b \otimes I_k)(\rho)\|_1$ , where  $I_k$  is the  $k$ -dimensional identity operation,

$\|\cdot\|_1$  denotes the trace norm, and the supremum is taken over all  $k \geq 1$  and density matrices  $\rho$  of dimension  $nk$ , with  $n$  the dimension of  $G_a$  and  $G_b$ . The diamond norm is also called the *completely bounded trace norm*, and plays the analogous role for quantum process distinguishability that the trace norm plays for density matrices. Specifically, the optimal probability of distinguishing  $G_a$  from  $G_b$  after a *single evaluation* is given by  $\frac{1}{2} + \frac{1}{4} \|G_a - G_b\|_\diamond$ .

4. **Frobenius-norm distance.** The Frobenius norm distance between two gates  $G_a$  and  $G_b$  is simply  $d_F = \sqrt{\text{Tr}[(G_a - G_b)^2]}$ . It has no known *operational* interpretation, but is very convenient as a rough measure of inaccuracy. It is also equal to the sum of the RMS errors in the individual matrix elements of the gates.

It’s also useful to know *how* the real gates (or, more precisely, GST’s estimates of the real gates) differ from the targets. There are several ways we could represent this, but the most useful involves an *error generator*. These are also given in Table 8. The final column of the table lists, for each gate, a Lindbladian superoperator  $\mathbb{L}$ . It is defined by the equation  $\hat{G} = G_{\text{target}} e^{\mathbb{L}}$ , where  $\hat{G}$  is the estimate and  $G_{\text{target}}$  is the ideal gate. This Lindbladian would be zero if the gates were perfect, and its overall magnitude is approximately equal to the diamond distance (or Jamiolkowski trace distance) between the target gate and the estimate.

| Gate | Process Infidelity | 1/2 Trace Distance | 1/2 $\diamond$ -Norm | Frobenius Distance |
|------|--------------------|--------------------|----------------------|--------------------|
| Gi   | 0.009114           | 0.016717           | 0.016826             | 0.038747           |
| Gx   | 0.001255           | 0.002925           | 0.002966             | 0.006301           |
| Gy   | 0.002082           | 0.003916           | 0.003925             | 0.009827           |

| Gate | Error Generator                                                                                                                                                                          |
|------|------------------------------------------------------------------------------------------------------------------------------------------------------------------------------------------|
| Gi   | $\begin{pmatrix} 0 & 0 & 0 & 0 \\ 0.0001 & -0.0212 & -0.0137 & 0.0021 \\ -0.0002 & 0.0258 & -0.0144 & -0.0017 \\ 0.0002 & 0.0036 & -0.0009 & -0.0008 \end{pmatrix}$                      |
| Gx   | $\begin{pmatrix} 0 & 0 & 0 & 0 \\ 6 \times 10^{-6} & 2 \times 10^{-5} & 0.0021 & -0.0005 \\ -0.0002 & -0.0008 & -0.0023 & -0.0019 \\ 0.0002 & -0.0034 & -0.0025 & -0.0028 \end{pmatrix}$ |
| Gy   | $\begin{pmatrix} 0 & 0 & 0 & 0 \\ -0.0002 & -0.0045 & 0.0013 & 0.005 \\ -2 \times 10^{-5} & 0.0042 & 0.0002 & 0.0003 \\ -0.0002 & -0.0023 & 0.0032 & -0.004 \end{pmatrix}$               |

Table 8: **Comparison of GST estimated gates to target gates.** This table presents, for each of the gates, three different measures of distance or discrepancy from the GST estimate to the ideal target operation. See text for more detail. The second table lists the “Error Generator” for each gate, which is the Lindbladian  $\mathbb{L}$  that describes *how* the gate is failing to match the target. This error generator is defined by the equation  $\hat{G} = G_{\text{target}} e^{\mathbb{L}}$ .

It’s usually useful to understand *how* gates fail. The error generators in Table 8 provide one view on this, but they are not necessarily intuitive. For example, you might want to know whether your gate suffers depolarizing, dephasing, or over-rotation errors. In Table 9, the estimated gates are decomposed into: (1) rotations (including angle and axis errors); (2) incoherent *diagonal* decay rates (depolarizing or  $T_1$  noise); and (3) incoherent *off-diagonal* decay rates (dephasing or  $T_2$  noise). These analyses can be compared with a the similar decomposition of the target gates (cf. table 2). Note that for some erroneous gates, this decomposition simply fails; if the numbers make no sense, this is probably the case.

It might be useful to know the closest *unitary* operation to the estimated gate, and how close it is. Usually, you were trying to implement a unitary. If the closest unitary to  $G$  was indeed  $G_{\text{target}}$ , then all

| Gate | Eigenvalues       | Fixed pt            | Rotn. axis | Diag. decay | Off-diag. decay |
|------|-------------------|---------------------|------------|-------------|-----------------|
| Gi   | 0.9995            | 0.8727              | 0          | 0.000545    | 0.01779         |
|      | $0.9822e^{i0.0}$  | 0.0325              | -0.0807    |             |                 |
|      | $0.9822e^{-i0.0}$ | 0.0044              | -0.0291    |             |                 |
|      | 1                 | 0.3317              | -0.9963    |             |                 |
| Gx   | $0.9975e^{i1.6}$  | 1                   | 0          | -0.000019   | 0.002521        |
|      | $0.9975e^{-i1.6}$ | $3 \times 10^{-7}$  | -1         |             |                 |
|      | 1                 | $-1 \times 10^{-5}$ | -0.0021    |             |                 |
|      | 1                 | -0.0002             | -0.0013    |             |                 |
| Gy   | $0.9957e^{i1.6}$  | 0.9913              | 0          | -0.000209   | 0.004265        |
|      | $0.9957e^{-i1.6}$ | 0.0001              | 0.0009     |             |                 |
|      | 1.0002            | 0.0929              | 1          |             |                 |
|      | 1                 | $-1 \times 10^{-5}$ | -0.0022    |             |                 |

| Gate | Angle         | Angle between Rotation Axes |               |               |
|------|---------------|-----------------------------|---------------|---------------|
|      |               | Gi                          | Gx            | Gy            |
| Gi   | $0.005852\pi$ |                             | $0.473843\pi$ | $0.508574\pi$ |
| Gx   | $0.499911\pi$ | $0.473843\pi$               |               | $0.500967\pi$ |
| Gy   | $0.501169\pi$ | $0.508574\pi$               | $0.500967\pi$ |               |

Table 9: **Eigen-decomposition of estimated gates.** Each estimated gate is described in terms of: (1) the eigenvalues of the superoperator; (2) the gate’s fixed point (as a vector in  $\mathcal{B}(\mathcal{H})$ , in the Pauli basis); (3) the axis around which it rotates, as a vector in  $\mathcal{B}(\mathcal{H})$ ; (4) the angle of the rotation that it applies; (5) the decay rate along the axis of rotation (“diagonal decay”); (6) the decay rate perpendicular to the axis of rotation (“off-diagonal decay”); and (7) the angle between each gate’s rotation axis and the rotation axes of the other gates. “X” indicates that the decomposition failed or couldn’t be interpreted.

errors are incoherent; if not, you might be able to tweak the gate parameters to get closer relatively easily. Also, implementing a particular unitary may be less important than just achieving *some* set of mutually independent unitaries. In these and other cases, the distance from an estimated gate to its closest unitary approximation is of interest.

Table 10 lists, for each estimated gate, the properties of its closest unitary approximation. The table defines the closest unitary, in terms of an axis and angle (in  $\mathcal{B}(\mathcal{H})$ ) of rotation. It also presents the process fidelity and Jamiolkowski trace distance between the estimated gate and its closest unitary approximation. A sanity check is computed by comparing the fidelity of the obtained closest unitary with a theoretical upper bound (if a value greater than one appears in this column then the other values in that row may be inaccurate). If these numbers are similar to those in Table 8, then the gates are as close to the targets as they are to *any* unitary.

Finally, Table 11 presents each estimated gate’s *Choi matrix*, along with its spectrum. The Choi matrix (sometimes ambiguously referred to as the “process matrix”) is an alternative way to describe a process. We usually prefer the “superoperator representation”, which has the very useful property that the process matrix corresponding to applying  $G_a$  and then  $G_b$  is simply  $G_b G_a$ . This is completely false for the Choi representation. Nonetheless, the Choi representation is often useful, so we present it here – but without a detailed discussion of its properties (see, e.g. the textbook by Nielsen and Chuang).

The Choi matrix  $\chi(G)$  for a gate  $G$  can be simply understood in either of two ways. First, it is equivalent (up to choice of basis) to the *Jamiolkowski state* defined by applying  $G$  to one half of a maximally entangled bipartite state. Second, it is the general (non-diagonal) form of the well-known Kraus representation,  $G[\rho] = \sum_i K_i \rho K_i^\dagger$ . The Choi matrix behaves in many ways like a quantum state, and appears naturally in expressions for the process fidelity and Jamiolkowski trace distance just as density matrices would enter these expressions when computing differences between states.

Additionally, the condition of *complete positivity* or CP (which all real quantum processes must satisfy) is simply the positivity of the Choi matrix. Thus, negative eigenvalues in Table 11 indicate that the estimate violates complete positivity. If they are very small, they may simply indicate statistical fluctuations (unitary

| Gate | Process Infidelity | 1/2 Trace Distance | Rotation Axis                             | Rotation Angle | Sanity ✓ |
|------|--------------------|--------------------|-------------------------------------------|----------------|----------|
| Gi   | 0.009018           | 0.012405           | 0<br>0.021<br>-0.039<br>0.999             | 0.006293 $\pi$ | 0.000001 |
| Gx   | 0.001254           | 0.002492           | 0<br>-1<br>-0.0014<br>$-5 \times 10^{-6}$ | 0.499911 $\pi$ | 0.000003 |
| Gy   | 0.002077           | 0.003185           | 0<br>0.0014<br>1<br>$5 \times 10^{-6}$    | 0.50117 $\pi$  | 0.000002 |

Table 10: Information pertaining to the closest unitary gate to each of the estimated gates.

gates have  $\chi$  matrices with zero eigenvalues, so any small fluctuation is likely to violate CP). If they are large, they serve as a warning that (1) the model of CPTP maps is probably violated (usually because of non-Markovian behavior), and (2) this estimate may produce negative or greater-than-unity probabilities. GST does *not* generally impose complete positivity (although it is an option), precisely because violation of CP is a warning flag for non-Markovian behavior (which is very common in experimental qubits).

| Gate | Choi matrix (Pauli basis)                                                                                                                                                                                                                                                               | Eigenvalues                            |
|------|-----------------------------------------------------------------------------------------------------------------------------------------------------------------------------------------------------------------------------------------------------------------------------------------|----------------------------------------|
| Gi   | $\begin{pmatrix} 0.9909 & 0.0002e^{-i1.5} & 0.0004e^{-i1.4} & 0.0097e^{-i1.6} \\ 0.0002e^{i1.5} & -0.0015 & 0.0029e^{-i3.1} & 0.0014e^{i0.0} \\ 0.0004e^{i1.4} & 0.0029e^{i3.1} & 0.0019 & 0.0006e^{-i0.0} \\ 0.0097e^{i1.6} & 0.0014e^{-i0.0} & 0.0006e^{i0.0} & 0.0087 \end{pmatrix}$ | -0.0034<br>0.0036<br>0.0088<br>0.991   |
| Gx   | $\begin{pmatrix} 0.5001 & 0.4987e^{-i1.6} & 0.0001e^{i0.9} & 0.0003e^{-i1.7} \\ 0.4987e^{i1.6} & 0.4999 & 0.0014e^{i3.1} & 0.0003e^{i3.0} \\ 0.0001e^{-i0.9} & 0.0014e^{-i3.1} & 0.0011 & 0.0001e^{-i3.1} \\ 0.0003e^{i1.7} & 0.0003e^{-i3.0} & 0.0001e^{i3.1} & -0.0011 \end{pmatrix}$ | -0.0012<br>0.0004<br>0.0021<br>0.9987  |
| Gy   | $\begin{pmatrix} 0.4982 & 0.0004e^{i1.7} & 0.4979e^{i1.6} & 0.0003e^{-i1.4} \\ 0.0004e^{-i1.7} & 0.0006 & 0.0018e^{-i3.1} & 0.0001e^{i0.0} \\ 0.4979e^{-i1.6} & 0.0018e^{i3.1} & 0.5019 & 0.0003e^{i0.2} \\ 0.0003e^{i1.4} & 0.0001e^{-i0.0} & 0.0003e^{-i0.2} & -0.0007 \end{pmatrix}$ | -0.0009<br>-0.0002<br>0.0032<br>0.9979 |

Table 11: **Choi matrix representation of the GST estimated gateset.** This table lists Choi representations of the estimated gates, and their eigenvalues. Unitary gates have a spectrum  $(1, 0, 0 \dots)$ , just like pure quantum states. Negative eigenvalues are non-physical, and may represent either statistical fluctuations or violations of the CPTP model used by GST.

## 4 Goodness-of-model Analysis

The previous section presented the estimated gateset, and compared it to the target gateset. This section is concerned with a mostly orthogonal analysis which seeks to explain how much the estimated gateset can be trusted – i.e., how well it fits the data.

To understand the goal of this section, consider the simple problem of fitting a line to a set of points. For any set of points, there is *always* a best-fit line – but this doesn’t mean that the best-fit line is a *good* fit! The data points may trace out a parabola, a square, or even something more complicated. It is essential to understand not just what the best-fit line was (and perhaps how close it was to some desired line), but

also **how well that linear model was able to fit all the data**. Of course, we do not expect it to fit every data point perfectly. The critical question is “Did the linear model fit *as well as we would expect it to* if the data really were generated by a linear process?”

In this analogy, GST’s estimated gateset is like the best-fit line, and the target gateset like the desired line. This section asks the question “How well was GST able to fit all of the data – and did it fit well enough to suggest that its model is valid?” A central tool used to do this is the *likelihood function*, which we denote  $\mathcal{L}$ , which formally is the probability of the observed data given a set of model parameters. The basic idea is that we maximize the likelihood function to obtain the best set of model parameters (i.e. gate set), and by looking at the value of this maximum we can determine the model’s goodness-of-fit. We will actually deal primarily with the logarithm of the likelihood function,  $\log(\mathcal{L})$ , which is similarly maximized.

#### 4.1 Aggregated $\log(\mathcal{L})$

The log-likelihood for an  $n$ -outcome system with predicted probabilities  $p_i$  and observed frequencies  $f_i$  ( $i = 1 \dots n$ ) is given by:

$$\log(\mathcal{L}) = \sum_i N f_i \log(p_i). \quad (1)$$

where  $N$  is the total number of counts. In *this* analysis,  $\log(\mathcal{L})$  is used to compare the set of probabilities predicted by a gateset ( $p_s$ ) and the frequencies obtained from a dataset ( $f_s$ ). Each experiment (or gate sequence)  $s$  is associated to two probabilities: “plus” has probability  $p_s$  and “minus” has probability  $1 - p_s$ . The  $\log(\mathcal{L})$  contribution of a single gate string  $s$  is

$$\log(\mathcal{L})_s = N f_s \log(p_s) + N(1 - f_s) \log(1 - p_s), \quad (2)$$

where  $N$  is the number of times the experiment  $s$  was performed,  $p_s$  is the probability of a “plus” outcome as predicted by the gateset, and  $f_s$  is the observed frequency of “plus”. The total log-likelihood for an entire dataset is just the sum

$$\log(\mathcal{L}) = \sum_{s \in \mathcal{S}} \log(\mathcal{L})_s. \quad (3)$$

A theoretical upper bound on the log-likelihood can be found by replacing  $p_s$  with  $f_s$  in Eq. 2 and evaluating Eq. 3. We will refer to this quantity as  $\log(\mathcal{L})_{ub}$ .

Statistical theory has quite a lot to say about the likelihood function (see any of the major textbooks). Using some of these results, we can predict that if there are  $N_p$  free parameters in the gateset that GST is fitting, and GST fits a dataset containing  $N_s > N_p$  distinct experiments (gate sequences), then *if the gateset model is correct*, then two times the difference between  $\log(\mathcal{L})_{ub}$  and the maximum  $\log(\mathcal{L})$  obtained is a random variable with a  $\chi_k^2$  distribution, where

$$k \equiv N_s - N_p.$$

Its expected value is  $\langle \chi^2 \rangle = k$ , and its RMS variance is  $\pm \sqrt{2k}$ . Thus, if the fit is “good”, then twice  $\Delta \log(\mathcal{L}) \equiv \log(\mathcal{L})_{ub} - \max(\log(\mathcal{L}))$  should lie roughly within the interval  $[k - \sqrt{2k}, k + \sqrt{2k}]$  where  $k = N_s - N_p$ . Thus, by comparing the difference  $2\Delta \log(\mathcal{L}) - k$  to  $\sqrt{2k}$  one can determine how well the GST estimate was able to fit the data in dataset “data\_fig2c-d”.

The MLEGST algorithm used to generate this estimate is iterative. It starts by fitting only data from the shortest gate sequences (which are easy to fit *and* insensitive to most non-Markovian noise), then successively adds longer and longer sequences (with base sequence length  $L \leq 1, 2, 4, 8, \dots$ ) to the mix. Since we get an estimate at each intermediate  $L$ , it is possible to quantify not just the goodness of the *best* fit (presented in the previous section), but how the goodness-of-fit behaves as longer and longer sequences are added in.

This data is presented in Table 12. What you should be looking for here is whether – at each value of  $L$  – the  $2\Delta \log(\mathcal{L})$  quantity is roughly the same as  $k$ . More precisely, is  $|2\Delta \log(\mathcal{L}) - k|$  less than or equal to  $\sqrt{2k}$ ? If not, then the model is not fitting as well as it should, which usually indicates non-Markovian noise (or, rarely, that the GST algorithm has simply failed to find a good fit even though one exists).

As a rough rule of thumb, for GST experiments involving relatively long sequences (e.g.  $L \geq 100$ ):

- “Incredibly good” (★★★★★) experiments have  $2\Delta \log(\mathcal{L}) \approx k$ , as predicted by theory (and seen in simulations).
- “Great” (★★★★) experiments have  $2\Delta \log(\mathcal{L}) \leq 2k$  or so.
- “Good” (★★★) experiments have  $2\Delta \log(\mathcal{L}) \leq 5k$  or so.
- “Okay” (★★) experiments have  $2\Delta \log(\mathcal{L}) \leq 10k$ .
- Experiments in which  $2\Delta \log(\mathcal{L}) > 10k$  (★) have very significant non-Markovian noise, and the results in the previous section should be viewed very cautiously.

| L   | $2\Delta \log(\mathcal{L})$ | $k$  | $2\Delta \log(\mathcal{L}) - k$ | $\sqrt{2k}$ | $P$                | $N_s$ | $N_p$ | Rating |
|-----|-----------------------------|------|---------------------------------|-------------|--------------------|-------|-------|--------|
| 0   | 104.9291                    | 61   | 43.92907                        | 11.04536    | $4 \times 10^{-4}$ | 92    | 31    | ★★★★★  |
| 1   | 104.9177                    | 61   | 43.91774                        | 11.04536    | $4 \times 10^{-4}$ | 92    | 31    | ★★★★★  |
| 2   | 362.15                      | 137  | 225.15                          | 16.55295    | 0                  | 168   | 31    | ★★★★★  |
| 4   | 1240.181                    | 410  | 830.181                         | 28.63564    | 0                  | 441   | 31    | ★★★    |
| 8   | 2760.762                    | 786  | 1974.762                        | 39.64846    | 0                  | 817   | 31    | ★★★    |
| 16  | 4878.05                     | 1170 | 3708.05                         | 48.37355    | 0                  | 1201  | 31    | ★★★    |
| 32  | 8384.233                    | 1554 | 6830.233                        | 55.74944    | 0                  | 1585  | 31    | ★★★    |
| 64  | 13042.85                    | 1938 | 11104.85                        | 62.25753    | 0                  | 1969  | 31    | ★★     |
| 128 | 17508.29                    | 2322 | 15186.29                        | 68.1469     | 0                  | 2353  | 31    | ★★     |
| 256 | 21281.8                     | 2706 | 18575.8                         | 73.5663     | 0                  | 2737  | 31    | ★★     |

Table 12: **Comparison between the computed and expected maximum  $\log(\mathcal{L})$  for different values of  $L$ .**  $N_s$  and  $N_p$  are the number of gate strings and parameters, respectively. The quantity  $2\Delta \log(\mathcal{L})$  measures the goodness of fit of the GST model (small is better) and is expected to lie within  $[k - \sqrt{2k}, k + \sqrt{2k}]$  where  $k = N_s - N_p$ .  $P$  is the p-value derived from a  $\chi_k^2$  distribution (i.e. when  $P <$  some threshold like 0.05 there is grounds for rejecting the GST fit). The rating from 1 to 5 stars gives a very crude indication of goodness of fit as explained in the text.

## 4.2 Detailed likelihood analysis

The aggregated  $2\Delta \log(\mathcal{L})$  numbers presented in Table 12 tell you how well the GST estimate fits the *entire* dataset. If they are in line with theory ( $2\Delta \log(\mathcal{L}) \approx k$ ), then there is little more to be said. But if the best fit to the data is not good, we can debug it by identifying *which* experiments are inconsistent with the fit.

Figure 1 displays the  $2\Delta \log(\mathcal{L})$  contribution from each individual gate sequence (Eq. 2). Each gate sequence corresponds to a single colored “pixel” in the plot. Each block of pixels corresponds to a single base sequence (i.e., a germ power), and the individual pixels within a block correspond to the various fiducial sequence pairs between which that base sequence was sandwiched. (The column indicates the fiducial adjacent to state preparation, while the row indicates the fiducial adjacent to measurement). Base sequences are arranged in a grid; different rows correspond to different germs, while different columns correspond to different maximum lengths  $L$ . Pixels are labeled with the  $2\Delta \log(\mathcal{L})$  contribution for that sequence, and colored appropriately. Shades of blue indicate  $2\Delta \log(\mathcal{L})$  contributions in the range 0-3 (“consistent”), while dark red indicates a  $2\Delta \log(\mathcal{L})$  contribution of 10 or above. Such events ( $2\Delta \log(\mathcal{L})_s \geq 10$ ) should occur only once per 638 experiments if the model is correct.

Identifying patterns and trends within such “pixel plots” can aid in identifying specific sources and types of non-Markovian noise which may be to blame if the GST algorithms are unable to produce a “good” estimate. For example, it is often the case that all the short sequences [ $L = O(1)$ ] can be fit reasonably well, but the right-hand side of Figure 1 becomes a sea of red. This indicates that non-Markovian behavior (potentially due to slow drift of gateset parameters) is becoming more significant for longer experiments. In other cases, a single row may be particularly bad, indicating that a particular gate or germ is especially problematic (e.g., was not stabilized using dynamical decoupling techniques). Be cautious in debugging,

however – sometimes bad  $\log(\mathcal{L})$  values for a particular gate or germ can result *not* from faults in that operation, but because another operation failed so badly that it distorted the entire fit (e.g., in trying to fit catastrophically non-Markovian data at Point A, GST ended up failing to fit perfectly good data at Point B).

If the “generate appendices” option was selected for this report, similar pixel plots for the intermediate estimates whose total  $2\Delta \log(\mathcal{L})$  is listed in Table 12 can be found in Appendix ??.

Figure 2 shows exactly the same  $\log(\mathcal{L})$  analysis as Figure 1, but arranged differently. Here, blocks (not square) all correspond to a single fiducial pair (e.g., pre- and post-fiducial), and pixels within a block correspond to different base sequences. This can be useful for diagnosing a single bad fiducial sequence.

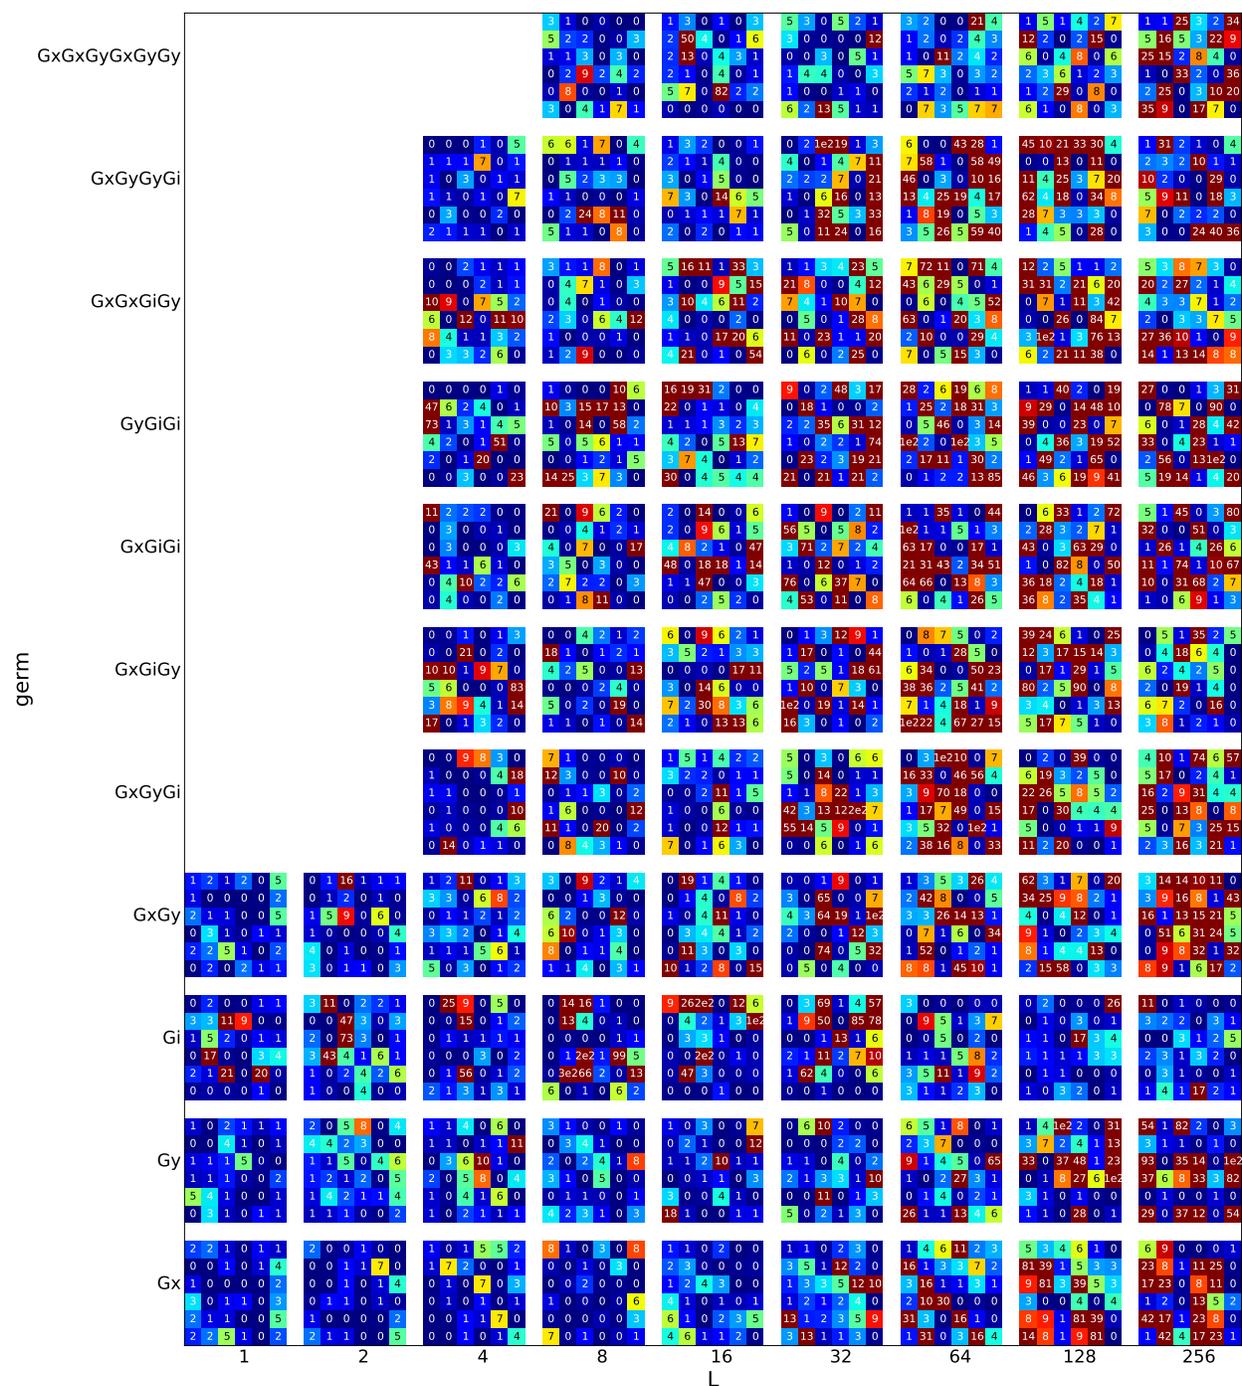

Figure 1:  $2\Delta\log(\mathcal{L})$  contributions for every individual experiment in the dataset. Each pixel represents a single experiment (gate sequence), and its color indicates whether GST was able to fit the corresponding frequency well. Blue is typical; dark red squares indicating  $2\Delta\log(\mathcal{L})_s > 10$  should appear only once per 638 experiments on average. Square blocks of pixels correspond to base sequences (arranged vertically by germ and horizontally by length); each pixel within a block corresponds to a specific choice of pre- and post-fiducial sequences. See text for further details.

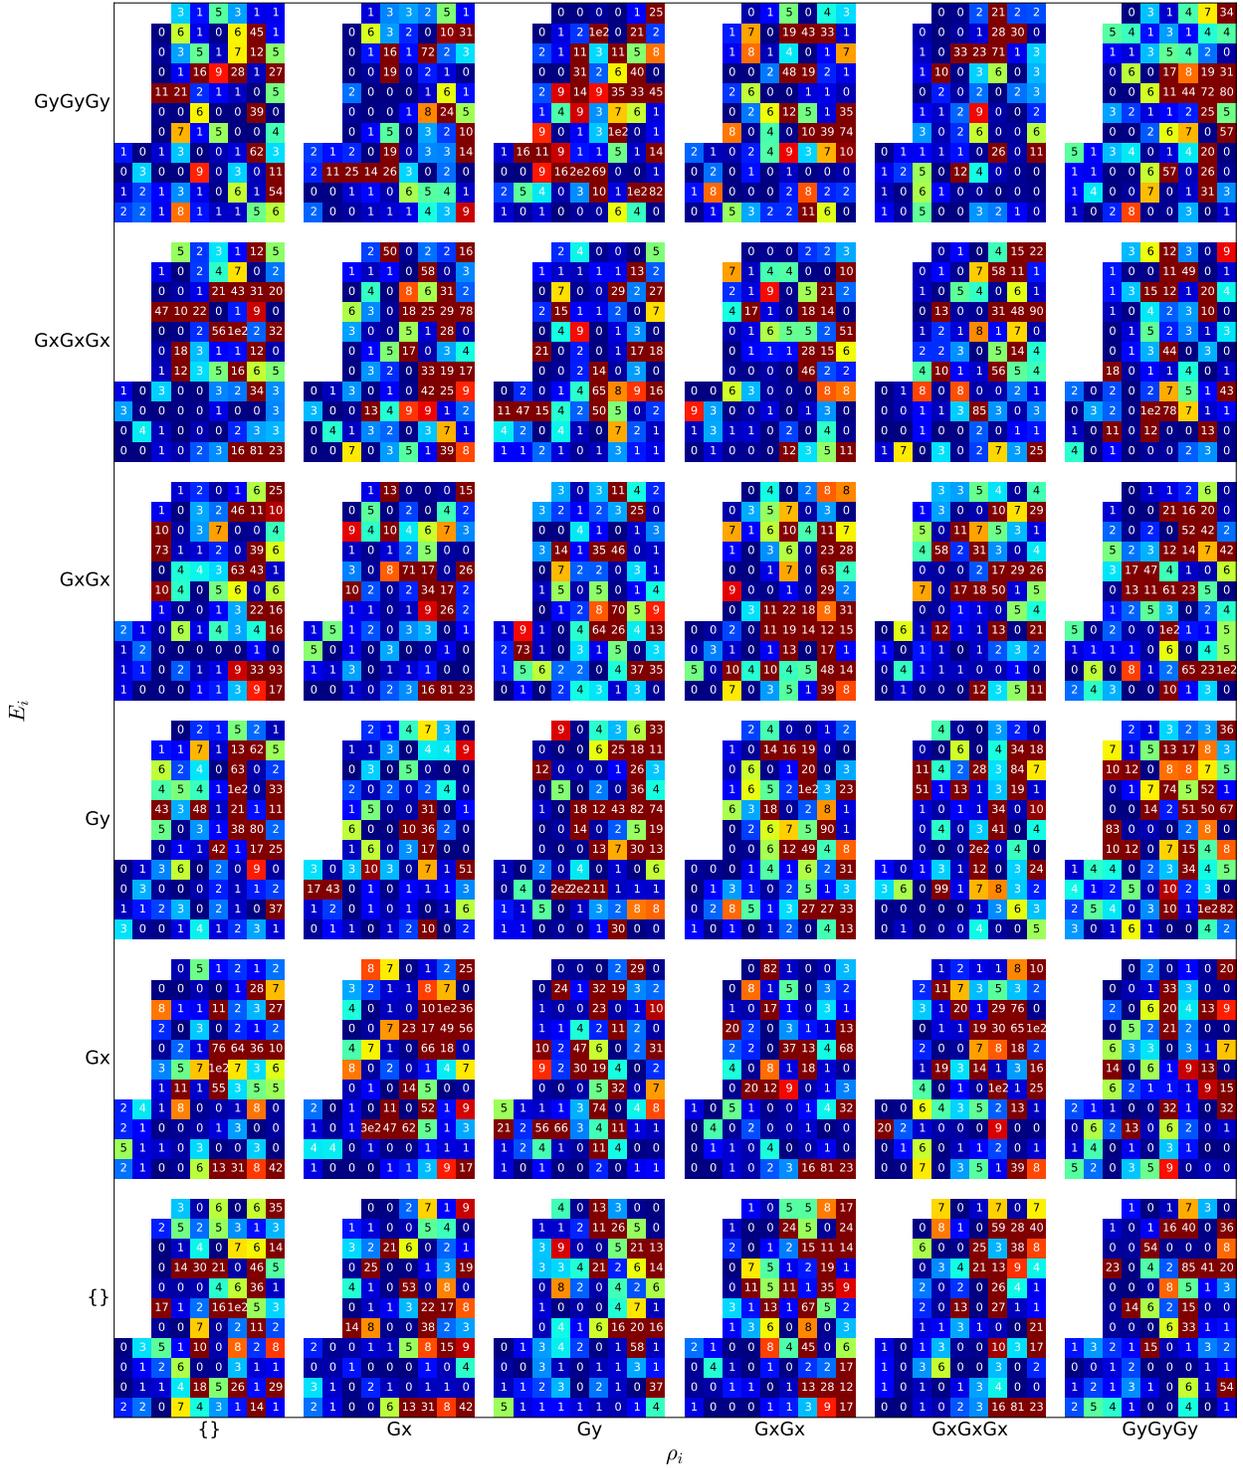

Figure 2:  $2\Delta \log(\mathcal{L})$  contributions for each experiment, arranged differently. This figure shows the same data as Figure 1, but arranged differently. Each block now corresponds to a particular pair of fiducial sequences, while pixels within the block correspond to different base sequences sandwiched between those fiducials.
